# Supplementary material for: Mini-o3: Scaling Up Reasoning Patterns and Interaction Turns for Visual Search
Source: arXiv:2509.07969 source file (2025-09-09)
Supplement: Supplementary file 1 [file appendix.tex]

\section{Data Setting Claim}
\label{app:data_setting}

In our preliminary experiments, we explored alternative data settings. Specifically, we conducted a comparative study on the \textbf{Qwen2.5 7B math base} model. The results indicated that models trained using data from the DAPO dataset yielded inferior performance compared to our current data configuration, which combines the \textbf{DeepScaler} and \textbf{SimpleRL} datasets. 

Consequently, we adopted the current setting for our main experiments. For the sake of experimental consistency and inertia, this data setting was maintained across all subsequent model training processes. However, it is important to note that this conclusion is based on our specific observations with the Qwen2.5 7B math base model. The findings may not be directly transferable or hold true for other base models, such as the \textbf{Qwen2.5 32B base}, which might exhibit different behaviors and data requirements.
